# Supplementary material for: High-yield fabrication of entangled photon emitters for hybrid quantum networking using high-temperature droplet epitaxy
Source: arXiv:1710.03483 ancillary file (2018-10-10)
Supplement: Supplementary file 1 [file suppinfo_FBassoBasset_High-yield_20181010.pdf]

# Supporting information: High-yield fabrication of entangled photon emitters for hybrid quantum networking using high-temperature droplet epitaxy

Francesco Basso Basset,<sup>\*,†,‡</sup> Sergio Bietti,<sup>†</sup> Marcus Reindl,<sup>‡</sup> Luca Esposito,<sup>†</sup>  
Alexey Fedorov,<sup>¶</sup> Daniel Huber,<sup>‡</sup> Armando Rastelli,<sup>‡</sup> Emiliano Bonera,<sup>†</sup> Rinaldo  
Trotta,<sup>\*,‡</sup> and Stefano Sanguinetti<sup>†,¶</sup>

<sup>†</sup>*L-NESS and Dipartimento di Scienza dei Materiali, Università degli Studi di  
Milano-Bicocca, Via Cozzi 55, I-20125 Milano, Italy*

<sup>‡</sup>*Institute of Semiconductor and Solid State Physics, Johannes Kepler University,  
Altenbergerstraße 69, Linz 4040, Austria*

<sup>¶</sup>*L-NESS and CNR-IFN, via Anzani 42, I-22100 Como, Italy*

E-mail: f.bassobasset@campus.unimib.it; rinaldo.trotta@jku.at

Phone: +39 02 64485157; +43 732 24689599

## Notes on morphological features

The AFM image from Fig. 1 (main text) is reported here in Fig. S1 using a different color scale. A contour map style is chosen to highlight how the planar section of the QD varies at different heights. As suggested in the main text, a very thin broad triangular base is visible, which is likely due to As incorporation in the near outside of the droplet. There, Ga adatom

concentration can be high enough to promote planar growth despite the low surface lifetime of As atoms. Further investigation will be needed to unravel the details of the crystallization dynamics.

Concerning the shape of the uncapped QD, the height profiles shown in Fig. 1b (main text) may suggest a rounded top. However, the image is limited by the resolution of the instrument, that in this case does not resolve atomic steps on the dot. The collection of morphology scans performed by AFM are actually compatible with a flat top picture.

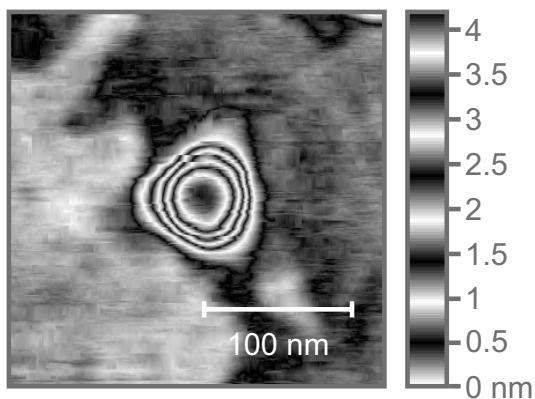

Figure S1: AFM scan of a typical single QD. A contour color scale is used in order to draw attention to sub-nanometer variations in height.

## Ensemble optical properties

Ensemble PL measurements were carried out by using the 532 nm line of a Nd:YAG continuous wave (CW) laser. The spectra reported here were acquired with a 0.5 mW excitation power on a spot with approximate diameter of 80  $\mu\text{m}$ . The sample temperature was kept at 16 K. The PL emission was dispersed by a 150 l/mm diffraction grating in a 500 mm focal length spectrometer and then analyzed by a Peltier cooled CCD detector.

Low temperature ensemble photoluminescence (PL) was employed to experimentally confirm the emission wavelength design. The exciting laser power was set low enough not to have an impact on the spectral shape. Under this condition, the contribution from excited

states recombination is negligible and the emission energy distribution reveals the actual population of fundamental excitonic states. It is possible to notice that it features sizable modulations which are typical of QDs with low aspect ratio and are caused by monolayer fluctuations in height.<sup>1-4</sup> The low energy part of the emission spectrum matches the 780 nm spectral window (see Fig. S2). The fact that the majority of the QDs on the investigated sample emit at lower wavelengths is not a drawback, because the surface density of emitters in the spectral region of interest is then low enough to allow for single dot spectroscopy without the need for spatial filters.

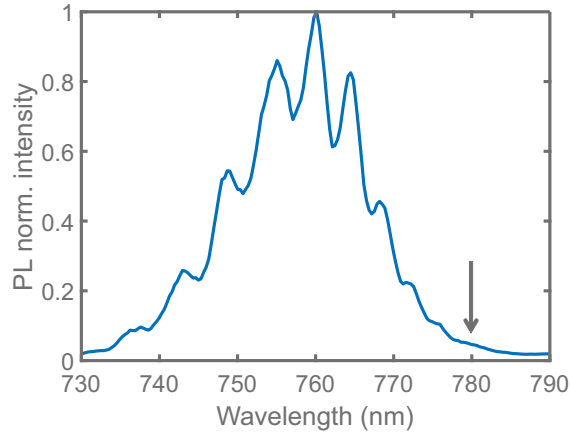

Figure S2: Low temperature ensemble PL spectrum of the sample investigated in the main text. The wavelength of  $^{87}\text{Rb}$  D<sub>2</sub> absorption lines is highlighted with a vertical arrow.

The ensemble PL signature did not change significantly after a post growth annealing (PGA) step at 700°C for 1 hour. We consider this as an additional evidence in favor of the beneficial effect of high temperature crystallization during the growth. Indeed, also the average zero-phonon exciton linewidth did not improve after this treatment, in contrast to what observed on samples fabricated with the standard DE process.<sup>5</sup> We suggest that the high crystalline quality of the samples obtained with this procedure reduces the concentration of point defects which facilitate interdiffusion processes at PGA temperatures and strongly contribute to spectral diffusion.

The main text focuses on the optical properties of the emitters in the spectral region relevant for interacting with Rb atomic clouds. In Fig. S3 we report experimental data for

FSS and radiative lifetime over the entire wavelength range of emission of the sample. While the radiative decay depends weakly on the exciton energy, the FSS increases markedly at higher energies. As mentioned in the main text, this behavior is attributed to the smaller size of the QDs, possibly because exchange interaction is enhanced by tighter carrier confinement,<sup>6</sup> and their shape is more strongly affected by minor anisotropies of the surface where the droplets are deposited. The in-plane orientation of the emitting dipole appears to be random, independently from the wavelength of emission.

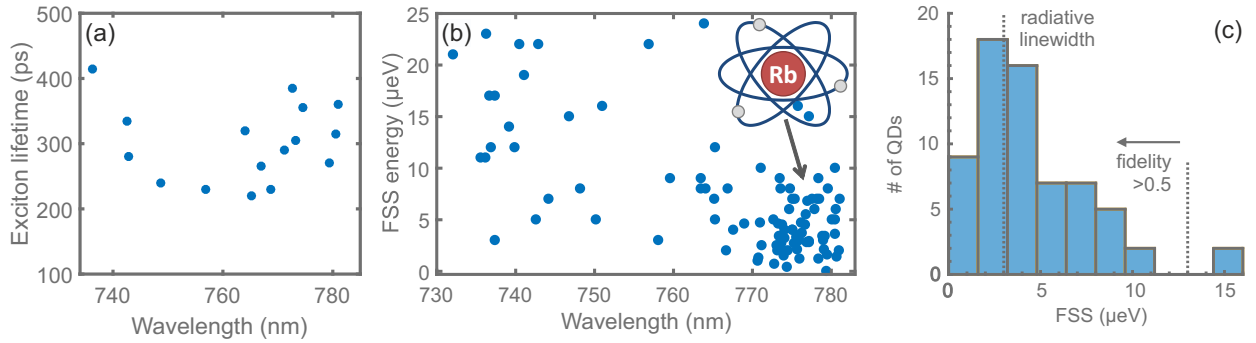

Figure S3: a) Exciton lifetime values measured on several QDs emitting at different wavelengths, estimated from the total decay time of the system under above-barrier excitation. b) FSS values measured on several QDs emitting at different wavelengths. c) Histogram of the fine structure splitting values from QDs emitting above 770 nm.

Fig. S3(c), also shown in the graphical abstract, collects in a histogram the distribution of fine structure splitting values from QDs emitting above 770 nm (see Fig. S3(b) or Fig. 2(c)). Other relevant figures of merit for entangled photon emission are displayed for immediate comparison, namely the typical radiative linewidth and the threshold for entanglement fidelity above the classical limit, as estimated with the exciton phase evolution model discussed in the main text.

## Excitonic complexes

The attribution of the observed emission lines to excitonic complexes is based on polarization-resolved measurements and confirmed by comparison with expected binding energies from

literature and by power dependence analysis.

In Fig. S4 a typical FSS measurement is shown, obtained by mapping the energy position of the exciton (X) and biexciton (XX) lines at different linear polarization angles. These two states display the distinctive polarization characteristics of the biexciton cascade,<sup>7</sup> since they recombine radiatively by emitting either of two orthogonal linearly polarized photons with slightly different energy. The exciton label is attributed to the more intense and higher energy line.

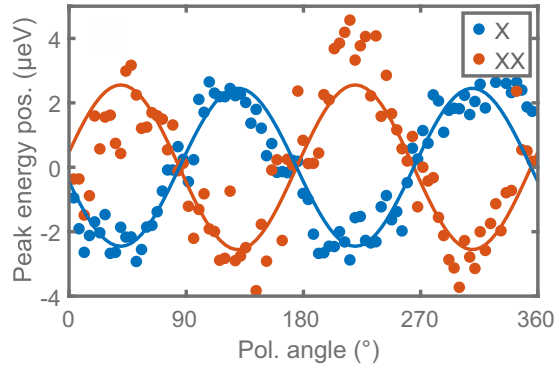

Figure S4: Emission energy of a pair of X and XX lines obtained by Gaussian fits of the spectra as a function of the polarization angle.

It is usually possible to spot one or two emission lines that show no dependence on linear polarization and high brightness at low excitation power. These are interpreted as radiative recombination from trion states (T). The attribution of the sign of the charge is not always immediate for bigger QDs, because of the presence of more than four emission lines at moderate laser power and their proximity in binding energy. In Fig. S5(a) it is reported the PL spectrum relative to a smaller QD, dominated by four emission lines. In this case, singly positively (X+) and negatively (X-) charged exciton can be identified, accordingly with typical binding energies from previous experimental<sup>8,9</sup> and theoretical studies.<sup>10</sup>

Power dependence analysis supports our interpretation, as the biexciton radiative recombination shows a clear quadratic dependency on the injection rate as compared to the exciton line. This was demonstrated quantitatively by using a random population model, where the PL intensity of exciton and biexciton follows a Poissonian dependence on the av-

erage occupation number inside the QD and on its square power respectively.<sup>11,12</sup> Numerical fits find good agreement with theory (experimental data points along with fitted curves are shown in Fig. S5(b)) and properly estimate a near one exponent in the power law for the dot population process. The power dependence of charged excitons emission on the photoinjected population may vary from linear to superlinear, as in the case of positively and negatively charged exciton respectively, depending on the leading capture mechanism of the extra charge.

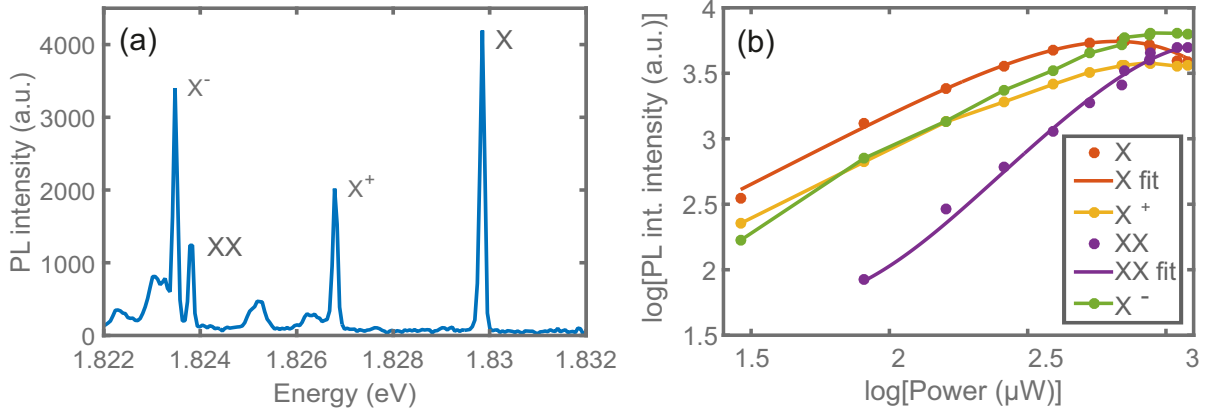

Figure S5: a) PL spectrum of a single QD with the main peaks labeled as recombination from specific excitonic complexes, consistently with polarization-resolved measurements and binding energy values. b) Power dependence of the PL intensities of the main lines of the spectrum shown in panel (a), along with numerical fits (continuous lines) for X and XX data points.

## Single photon purity

The second-order coherence function for X and XX radiative recombination was evaluated with a Hanbury-Brown-Twiss setup for photon correlation experiments. These measurements were performed to assess the quality of single photon emission under pulsed resonant two-photon excitation. The excitaton power was tuned to  $\pi$  pulse. An example of  $g^{(2)}(\tau)$  curve is reported in Fig. S6. The autocorrelation function at zero delay is  $0.03 \pm 0.01$  and  $0.05 \pm 0.02$  for X and XX emission respectively.  $g^{(2)}(0)$  is calculated by dividing the integrated intensity

of the zero delay peak by the average one of the side peaks, whereas the error is estimated by assuming Poissonian statistic on the number of avalanche photodiode counts. These values denote a high single photon purity, with a possible contribution from incomplete suppression of the background laser light. Such a result confirms that this excitation scheme is an improvement over above-barrier excitation, in which case the purity of the XX transition can be compromised by radiative recombination of other excitonic complexes with similar binding energies.

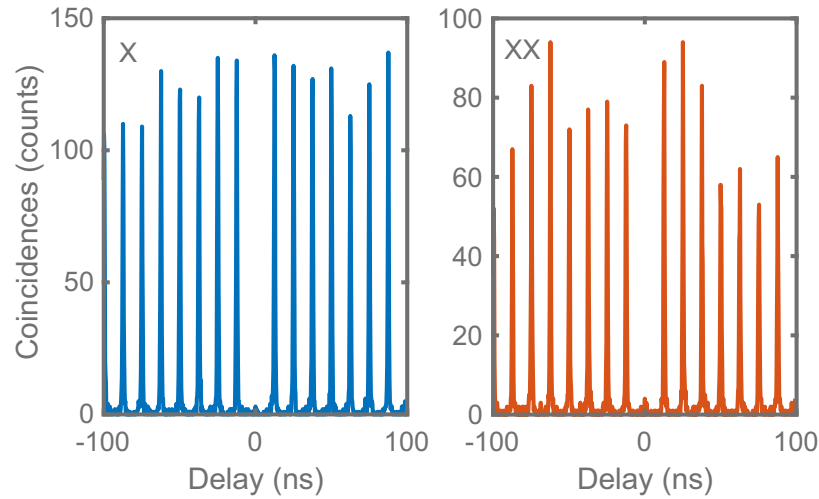

Figure S6: Auto-correlation function measurements of a typical quantum dot for the X and XX emission line, under  $\pi$  pulse resonant two-photon excitation.

## References

- (1) Sakuma, Y.; Takeguchi, M.; Takemoto, K.; Hirose, S.; Usuki, T.; Yokoyama, N. *J. Vac. Sci. Technol., B: Microelectron. Nanometer Struct.–Process., Meas., Phenom.* **2005**, *23*, 1741–1746.
- (2) Takaaki, M.; Marco, A.; Takashi, K.; Brian, M.; Akihiro, O.; Kazutaka, M.; Kazuaki, S. *Appl. Phys. Express* **2010**, *3*, 065203.
- (3) Guffarth, F.; Heitz, R.; Schliwa, A.; Ptschke, K.; Bimberg, D. *Phys. E (Amsterdam,*

- Neth.*) **2004**, *21*, 326 – 330, Proceedings of the Eleventh International Conference on Modulated Semiconductor Structures.
- (4) Wang, L.; Rastelli, A.; Schmidt, O. G. *J. Appl. Phys.* **2006**, *100*, 064313.
  - (5) Mano, T.; Abbarchi, M.; Kuroda, T.; Mastrandrea, C.; Vinattieri, A.; Sanguinetti, S.; Sakoda, K.; Gurioli, M. *Nanotechnology* **2009**, *20*, 395601.
  - (6) Huo, Y. H.; Krápek, V.; Rastelli, A.; Schmidt, O. G. *Phys. Rev. B* **2014**, *90*, 041304.
  - (7) Bayer, M.; Ortner, G.; Stern, O.; Kuther, A.; Gorbunov, A. A.; Forchel, A.; Hawrylak, P.; Fafard, S.; Hinzer, K.; Reinecke, T. L.; Walck, S. N.; Reithmaier, J. P.; Klopff, F.; Schäfer, F. *Phys. Rev. B* **2002**, *65*, 195315.
  - (8) Abbarchi, M.; Mastrandrea, C. A.; Kuroda, T.; Mano, T.; Sakoda, K.; Koguchi, N.; Sanguinetti, S.; Vinattieri, A.; Gurioli, M. *Phys. Rev. B* **2008**, *78*, 125321.
  - (9) Bouet, L.; Vidal, M.; Mano, T.; Ha, N.; Kuroda, T.; Durnev, M. V.; Glazov, M. M.; Ivchenko, E. L.; Marie, X.; Amand, T.; Sakoda, K.; Wang, G.; Urbaszek, B. *Appl. Phys. Lett.* **2014**, *105*, 082111.
  - (10) Luo, J.-W.; Zunger, A. *Phys. Rev. B* **2011**, *84*, 235317.
  - (11) Grundmann, M.; Bimberg, D. *Phys. Rev. B* **1997**, *55*, 9740–9745.
  - (12) Abbarchi, M.; Mastrandrea, C.; Kuroda, T.; Mano, T.; Vinattieri, A.; Sakoda, K.; Gurioli, M. *J. Appl. Phys.* **2009**, *106*, 053504.
